# Supplementary material for: Spherical Geometry and the Least Symmetric Triangle
Source: arXiv:1708.01559 ancillary file (2017-08-03)
Supplement: Supplementary file 1 [file ScaleneTriangles.pdf]

# Spherical Geometry and the Most Scalene Triangle

## Supplementary Materials

— Laney Bowden, Andrea Haynes, Clayton Shonkwiler, and Aaron Shukert

## Most scalene obtuse triangle

As explained in the text of the paper, the most scalene obtuse triangle corresponds to a point on the sphere which must lie on the
curve

$$p(t) = \cos(t)\left(\frac{1}{\sqrt{2}}, \frac{1}{\sqrt{2}}, 0\right) + \sin(t)\left(\frac{1}{2}, \frac{-1}{2}, \frac{1}{\sqrt{2}}\right) = \left(\frac{\sqrt{2}\,\cos(t)+\sin(t)}{2}, \frac{\sqrt{2}\,\cos(t)-\sin(t)}{2}, \frac{\sin(t)}{\sqrt{2}}\right).$$

```
p[t_] := {(Sqrt[2] Cos[t] + Sin[t]) / 2, (Sqrt[2] Cos[t] - Sin[t]) / 2, Sin[t] / Sqrt[2]};
```

On the other hand, the right triangles lie on the curve

$$q(x) = \left(x, \sqrt{\frac{1-x^2}{1+x^2}}, x\sqrt{\frac{1-x^2}{1+x^2}}\right)$$

```
q[x_] := {x, Sqrt[(1 - x^2) / (1 + x^2)], x Sqrt[(1 - x^2) / (1 + x^2)]};
```

We see that the distance from $p(t)$ to $q(x)$ is

```
ArcCos[p[t].q[x]]
```

$$\text{ArcCos}\left[\frac{1}{2}\sqrt{\frac{1-x^2}{1+x^2}}\left(\sqrt{2}\,\text{Cos}[t]-\text{Sin}[t]\right)+\frac{x\sqrt{\frac{1-x^2}{1+x^2}}\,\text{Sin}[t]}{\sqrt{2}}+\frac{1}{2}\,x\left(\sqrt{2}\,\text{Cos}[t]+\text{Sin}[t]\right)\right]$$

and the challenge is to determine when this quantity equals $\arcsin\left(\frac{\sin(t)}{\sqrt{2}}\right) = \arccos\left(\frac{\sqrt{3+\cos(2\,s)}}{2}\right)$. After eliminating the inverse cosines, we are solving

```
sols = Solve[1/2 Sqrt[(1 - x^2)/(1 + x^2)] (Sqrt[2] Cos[t] - Sin[t]) +
   (x Sqrt[(1-x^2)/(1+x^2)] Sin[t])/Sqrt[2] + 1/2 x (Sqrt[2] Cos[t] + Sin[t]) == Sqrt[3 + Cos[2 t]]/2, x]
```

```
{{x → -((-2 √2 Cos[t] √(3 + Cos[2 t]) + 4 Cos[t] Sin[t] - 2 √(3 + Cos[2 t]) Sin[t] -
      2 √2 Sin[t]^2) / (4 (2 Cos[t]^2 + 2 √2 Cos[t] Sin[t] + 3 Sin[t]^2))) -
   1/2 √((6 Cos[t]^2)/(… 1 …)^2 + (2 … 1 …^2 Cos[2 t])/(… 1 …)^2 + … 29 … + (… 1 …)^(1/3)/(3 × 2^(1/3))) -
   1/2 √(… 42 … + (… 1 …)/(… 1 …) - (… 1 …)^(1/3)/(3 × 2^(1/3)) - (-((8 (-2 √2 Cos[t] √(3 + Cos[2 t]) -
        4 Cos[t] Sin[t] - … 1 … + 2 √2 Sin[t]^2)) / (2 Cos[t]^2 +
        2 √2 Cos[t] Sin[t] + 3 Sin[t]^2)) + ((… 1 …) (… 1 …))/(2 … 1 …^2 + … 1 … + 3 … 1 …)) /
     (4 √((6 Cos[t]^2)/(2 … 1 …^2 + … 1 … + 3 … 1 …)^2 + (2 Cos[t]^2 Cos[2 t])/(… 1 …)^2 + … 29 … + (… 1 …)^(1/3)/(3 × 2^(1/3)))))},
 … 2 …, {x → -(… 1 …)/(4 … 1 …) + … 1 … + … 1 …}}
```

large output | show less | show more | show all | set size limit...

There are four solutions above, but two are always complex and two are sometimes complex and sometimes real. Now, we're after the smallest value of *t* that gives a possible solution, which is to say, a real value of *x*, so this will be the value of *t* where two (conjugate) complex solutions become real and then bifurcate, which we see happens in the plot at a value of *t* slightly smaller than 0.3.

```
Plot[Evaluate[x /. # & /@ sols], {t, 0, π/8}]
```

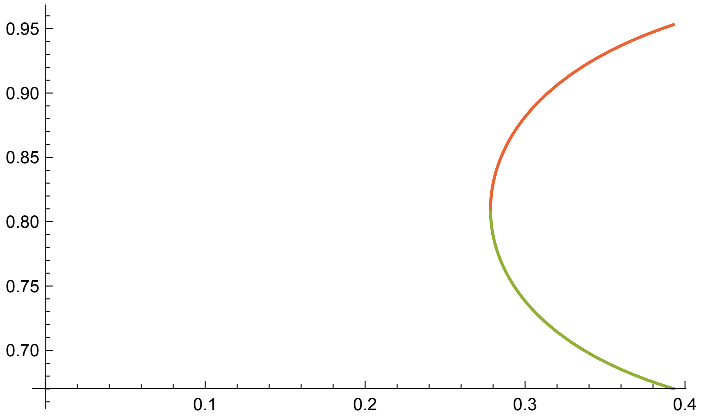


Based on *Mathematica*'s default color scheme, we can see that these are the third and fourth solutions found above, so the value of *t* we want is the one where the following function switches from complex to real:

```
x /. sols[[3]]
```

```
-((-2 √2 Cos[t] √(3 + Cos[2 t]) + 4 Cos[t] Sin[t] - 2 √(3 + Cos[2 t]) Sin[t] -
      2 √2 Sin[t]^2) / (4 (2 Cos[t]^2 + 2 √2 Cos[t] Sin[t] + 3 Sin[t]^2))) +
 1/2 √(6 … 1 …^2/(… 1 …)^2 + … 30 … + … 1 … … 1 …/(3 … 1 …)) - 1/2 √(… 45 … + (-8 (… 1 …)/… 1 … + … 1 …/… 1 …)/(4 √(6 … 1 …/… 1 …^2 + … 31 …)))

large output | show less | show more | show all | set size limit...
```

The above is the sum of three functions: a fraction and two square roots. The only term that is problematic is the last square root: the term under the square root can be negative. So we extract the term under the last square root:

```
complexterm = %[[3, 2, 1]]
```

```
… 45 … + (-8 (… 1 …)/(2 Cos … 1 … … 1 …]^2 + … 1 … +3 … 1 …) + … 1 … … 1 … … 1 …/… 1 …)/(4 √(6 Cos[t]^2/(… 1 …)^2 + … 1 …/… 1 …^2 + … 29 … + (… 1 …)^(1/3)/(3 × 2 … 1 …)))

large output | show less | show more | show all | set size limit...
```

The value of *t* that we want is the root of this expression:

```
Plot[complexterm, {t, 0, π/8}]
```

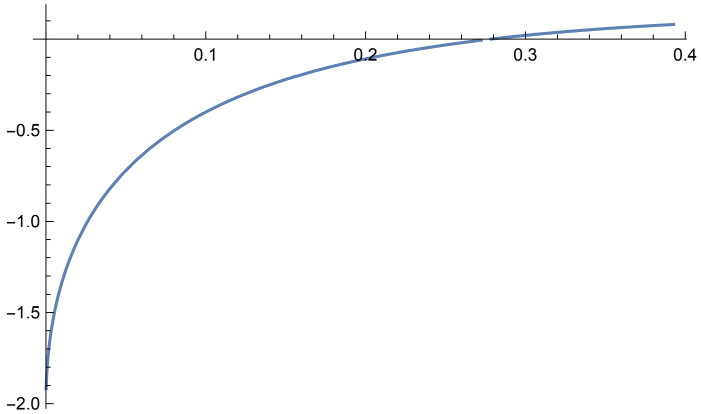


There are (by *Mathematica*'s count) 28 terms in this expression:

```
Length[complexterm]
```

```
28
```

And, of those 28, terms 17–27 can be complex, which we can verify by evaluating them at a value of *t* smaller then the value where they become real; say at $t = 0.1$.

```
TableForm[Table[{i, Chop[complexterm[[i]] /. t → 0.2]}, {i, 1, 28, 1}]]
```

| | |
|---|---|
| 1 | -0.859012 |
| 2 | -0.263734 |
| 3 | -0.246257 |
| 4 | -0.075606 |
| 5 | 0.318607 |
| 6 | -0.017649 |
| 7 | -0.0226032 |
| 8 | -0.0054186 |
| 9 | 0.00647977 |
| 10 | -0.006546 |
| 11 | -0.000464398 |
| 12 | 0.772144 |
| 13 | 0.988891 |
| 14 | 0.237064 |
| 15 | -5.9943 |
| 16 | 3.51661 |
| 17 | -0.232023 + 0.0925673 i |
| 18 | -0.594307 + 0.237103 i |
| 19 | 0.761133 - 0.30366 i |
| 20 | -0.142472 + 0.0568401 i |
| 21 | -0.182464 + 0.0727955 i |
| 22 | -0.0218708 + 0.00872553 i |
| 23 | -0.0732627 + 0.0292287 i |
| 24 | -0.046914 + 0.0187167 i |
| 25 | -0.0224931 + 0.0089738 i |
| 26 | 0.00048194 - 0.000192274 i |
| 27 | -0.554191 - 0.221099 i |
| 28 | 2.65178 |

Each of these potentially-complex terms switches from complex to real at the same time the overall function switches from negative to positive.

```
Plot[
 Evaluate@Prepend[Table[complexterm[[i]], {i, 17, 27}], complexterm], {t, 0, π/8}]
```

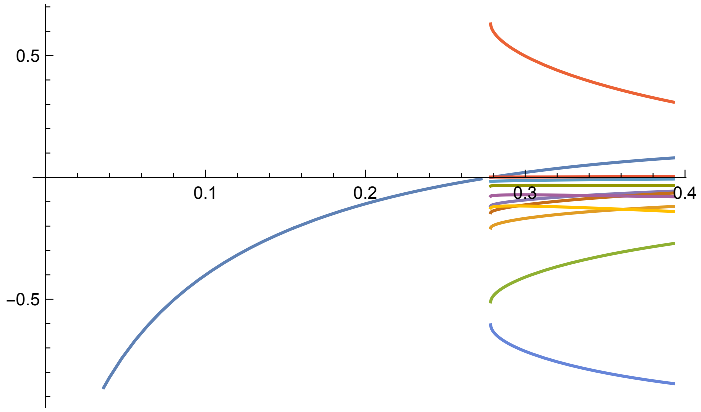


So we can focus on a single term to see when it stops being complex:

```
complexterm[[17]]
```

$$-\left((3\times 2^{1/3}) \Big/ \left((2\,\mathrm{Cos}[t]^2+2\sqrt{2}\,\mathrm{Cos}[t]\,\mathrm{Sin}[t]+3\,\mathrm{Sin}[t]^2)^2\right.\right.$$

$$
\Bigg(\frac{54}{\left(2\,\text{Cos}[t]^2+2\sqrt{2}\,\text{Cos}[t]\,\text{Sin}[t]+3\,\text{Sin}[t]^2\right)^3}+
$$

$$
\frac{216\,\text{Cos}[t]^2}{\left(2\,\text{Cos}[t]^2+2\sqrt{2}\,\text{Cos}[t]\,\text{Sin}[t]+3\,\text{Sin}[t]^2\right)^3}-
$$

$$
\frac{1440\,\text{Cos}[t]^4}{\left(2\,\text{Cos}[t]^2+2\sqrt{2}\,\text{Cos}[t]\,\text{Sin}[t]+3\,\text{Sin}[t]^2\right)^3}+
$$

$$
\frac{1280\,\text{Cos}[t]^6}{\left(2\,\text{Cos}[t]^2+2\sqrt{2}\,\text{Cos}[t]\,\text{Sin}[t]+3\,\text{Sin}[t]^2\right)^3}+
$$

$$
\frac{54\,\text{Cos}[2\,t]}{\left(2\,\text{Cos}[t]^2+2\sqrt{2}\,\text{Cos}[t]\,\text{Sin}[t]+3\,\text{Sin}[t]^2\right)^3}+
$$

$$
\frac{144\,\text{Cos}[t]^2\,\text{Cos}[2\,t]}{\left(2\,\text{Cos}[t]^2+2\sqrt{2}\,\text{Cos}[t]\,\text{Sin}[t]+3\,\text{Sin}[t]^2\right)^3}-
$$

$$
\frac{480\,\text{Cos}[t]^4\,\text{Cos}[2\,t]}{\left(2\,\text{Cos}[t]^2+2\sqrt{2}\,\text{Cos}[t]\,\text{Sin}[t]+3\,\text{Sin}[t]^2\right)^3}+
$$

$$
\frac{18\,\text{Cos}[2\,t]^2}{\left(2\,\text{Cos}[t]^2+2\sqrt{2}\,\text{Cos}[t]\,\text{Sin}[t]+3\,\text{Sin}[t]^2\right)^3}+
$$

$$
\frac{24\,\text{Cos}[t]^2\,\text{Cos}[2\,t]^2}{\left(2\,\text{Cos}[t]^2+2\sqrt{2}\,\text{Cos}[t]\,\text{Sin}[t]+3\,\text{Sin}[t]^2\right)^3}+
$$

$$
\frac{2\,\text{Cos}[2\,t]^3}{\left(2\,\text{Cos}[t]^2+2\sqrt{2}\,\text{Cos}[t]\,\text{Sin}[t]+3\,\text{Sin}[t]^2\right)^3}-
$$

$$
\frac{1296\sqrt{2}\,\text{Cos}[t]^2\sqrt{3+\text{Cos}[2\,t]}\,\text{Sin}[t]}{\left(2\,\text{Cos}[t]^2+2\sqrt{2}\,\text{Cos}[t]\,\text{Sin}[t]+3\,\text{Sin}[t]^2\right)^3}+
$$

$$
\frac{1728\sqrt{2}\,\text{Cos}[t]^4\sqrt{3+\text{Cos}[2\,t]}\,\text{Sin}[t]}{\left(2\,\text{Cos}[t]^2+2\sqrt{2}\,\text{Cos}[t]\,\text{Sin}[t]+3\,\text{Sin}[t]^2\right)^3}-
$$

$$
\frac{432\sqrt{2}\,\text{Cos}[t]^2\,\text{Cos}[2\,t]\sqrt{3+\text{Cos}[2\,t]}\,\text{Sin}[t]}{\left(2\,\text{Cos}[t]^2+2\sqrt{2}\,\text{Cos}[t]\,\text{Sin}[t]+3\,\text{Sin}[t]^2\right)^3}-
$$

$$
\frac{1296\,\text{Sin}[t]^2}{\left(2\,\text{Cos}[t]^2+2\sqrt{2}\,\text{Cos}[t]\,\text{Sin}[t]+3\,\text{Sin}[t]^2\right)^3}+
$$

$$
\frac{5184\,\text{Cos}[t]^2\,\text{Sin}[t]^2}{\left(2\,\text{Cos}[t]^2+2\sqrt{2}\,\text{Cos}[t]\,\text{Sin}[t]+3\,\text{Sin}[t]^2\right)^3}+
$$

$$
\frac{576\,\text{Cos}[t]^4\,\text{Sin}[t]^2}{\left(2\,\text{Cos}[t]^2+2\sqrt{2}\,\text{Cos}[t]\,\text{Sin}[t]+3\,\text{Sin}[t]^2\right)^3}-
$$

$$
\frac{864\,\text{Cos}[2\,t]\,\text{Sin}[t]^2}{\left(2\,\text{Cos}[t]^2+2\sqrt{2}\,\text{Cos}[t]\,\text{Sin}[t]+3\,\text{Sin}[t]^2\right)^3}+
$$

$$
\frac{1728\,\text{Cos}[t]^2\,\text{Cos}[2\,t]\,\text{Sin}[t]^2}{\left(2\,\text{Cos}[t]^2+2\sqrt{2}\,\text{Cos}[t]\,\text{Sin}[t]+3\,\text{Sin}[t]^2\right)^3}-
$$

$$
\frac{144\,\text{Cos}[2\,t]^2\,\text{Sin}[t]^2}{\left(2\,\text{Cos}[t]^2+2\sqrt{2}\,\text{Cos}[t]\,\text{Sin}[t]+3\,\text{Sin}[t]^2\right)^3}+
$$

$$\frac{648\sqrt{2}\,\sqrt{3+\text{Cos}[2\,t]}\,\text{Sin}[t]^3}{\left(2\,\text{Cos}[t]^2+2\sqrt{2}\,\text{Cos}[t]\,\text{Sin}[t]+3\,\text{Sin}[t]^2\right)^3}+$$

$$\frac{864\sqrt{2}\,\text{Cos}[t]^2\sqrt{3+\text{Cos}[2\,t]}\,\text{Sin}[t]^3}{\left(2\,\text{Cos}[t]^2+2\sqrt{2}\,\text{Cos}[t]\,\text{Sin}[t]+3\,\text{Sin}[t]^2\right)^3}+$$

$$\frac{216\sqrt{2}\,\text{Cos}[2\,t]\sqrt{3+\text{Cos}[2\,t]}\,\text{Sin}[t]^3}{\left(2\,\text{Cos}[t]^2+2\sqrt{2}\,\text{Cos}[t]\,\text{Sin}[t]+3\,\text{Sin}[t]^2\right)^3}+$$

$$\frac{2160\,\text{Sin}[t]^4}{\left(2\,\text{Cos}[t]^2+2\sqrt{2}\,\text{Cos}[t]\,\text{Sin}[t]+3\,\text{Sin}[t]^2\right)^3}-$$

$$\frac{1440\,\text{Cos}[t]^2\,\text{Sin}[t]^4}{\left(2\,\text{Cos}[t]^2+2\sqrt{2}\,\text{Cos}[t]\,\text{Sin}[t]+3\,\text{Sin}[t]^2\right)^3}+$$

$$\frac{720\,\text{Cos}[2\,t]\,\text{Sin}[t]^4}{\left(2\,\text{Cos}[t]^2+2\sqrt{2}\,\text{Cos}[t]\,\text{Sin}[t]+3\,\text{Sin}[t]^2\right)^3}-$$

$$\frac{864\sqrt{2}\,\sqrt{3+\text{Cos}[2\,t]}\,\text{Sin}[t]^5}{\left(2\,\text{Cos}[t]^2+2\sqrt{2}\,\text{Cos}[t]\,\text{Sin}[t]+3\,\text{Sin}[t]^2\right)^3}+$$

$$\frac{432\,\text{Sin}[t]^6}{\left(2\,\text{Cos}[t]^2+2\sqrt{2}\,\text{Cos}[t]\,\text{Sin}[t]+3\,\text{Sin}[t]^2\right)^3}+$$

$$\sqrt{}\Big(\Big(4\,\big(-9-24\,\text{Cos}[t]^2+32\,\text{Cos}[t]^4-6\,\text{Cos}[2\,t]-8\,\text{Cos}[t]^2\,\text{Cos}[2\,t]-\text{Cos}[2\,t]^2-$$

$$72\,\text{Sin}[t]^2-48\,\text{Cos}[t]^2\,\text{Sin}[t]^2-24\,\text{Cos}[2\,t]\,\text{Sin}[t]^2+12\,\text{Sin}[t]^4\big)^3\Big)\Big/$$

$$\left(2\,\text{Cos}[t]^2+2\sqrt{2}\,\text{Cos}[t]\,\text{Sin}[t]+3\,\text{Sin}[t]^2\right)^6+$$

$$\Big(54\Big/\left(2\,\text{Cos}[t]^2+2\sqrt{2}\,\text{Cos}[t]\,\text{Sin}[t]+3\,\text{Sin}[t]^2\right)^3+$$

$$\left(216\,\text{Cos}[t]^2\right)\Big/\left(2\,\text{Cos}[t]^2+2\sqrt{2}\,\text{Cos}[t]\,\text{Sin}[t]+3\,\text{Sin}[t]^2\right)^3-$$

$$\left(1440\,\text{Cos}[t]^4\right)\Big/\left(2\,\text{Cos}[t]^2+2\sqrt{2}\,\text{Cos}[t]\,\text{Sin}[t]+3\,\text{Sin}[t]^2\right)^3+$$

$$\left(1280\,\text{Cos}[t]^6\right)\Big/\left(2\,\text{Cos}[t]^2+2\sqrt{2}\,\text{Cos}[t]\,\text{Sin}[t]+3\,\text{Sin}[t]^2\right)^3+$$

$$\left(54\,\text{Cos}[2\,t]\right)\Big/\left(2\,\text{Cos}[t]^2+2\sqrt{2}\,\text{Cos}[t]\,\text{Sin}[t]+3\,\text{Sin}[t]^2\right)^3+$$

$$\left(144\,\text{Cos}[t]^2\,\text{Cos}[2\,t]\right)\Big/\left(2\,\text{Cos}[t]^2+2\sqrt{2}\,\text{Cos}[t]\,\text{Sin}[t]+3\,\text{Sin}[t]^2\right)^3-$$

$$\left(480\,\text{Cos}[t]^4\,\text{Cos}[2\,t]\right)\Big/\left(2\,\text{Cos}[t]^2+2\sqrt{2}\,\text{Cos}[t]\,\text{Sin}[t]+3\,\text{Sin}[t]^2\right)^3+$$

$$\left(18\,\text{Cos}[2\,t]^2\right)\Big/\left(2\,\text{Cos}[t]^2+2\sqrt{2}\,\text{Cos}[t]\,\text{Sin}[t]+3\,\text{Sin}[t]^2\right)^3+$$

$$\left(24\,\text{Cos}[t]^2\,\text{Cos}[2\,t]^2\right)\Big/\left(2\,\text{Cos}[t]^2+2\sqrt{2}\,\text{Cos}[t]\,\text{Sin}[t]+3\,\text{Sin}[t]^2\right)^3+$$

$$\left(2\,\text{Cos}[2\,t]^3\right)\Big/\left(2\,\text{Cos}[t]^2+2\sqrt{2}\,\text{Cos}[t]\,\text{Sin}[t]+3\,\text{Sin}[t]^2\right)^3-$$

$$\left(1296\sqrt{2}\,\text{Cos}[t]^2\sqrt{3+\text{Cos}[2\,t]}\,\text{Sin}[t]\right)\Big/\Big(2\,\text{Cos}[t]^2+2\sqrt{2}\,\text{Cos}[t]$$

$$\text{Sin}[t]+3\,\text{Sin}[t]^2\Big)^3+\Big(1728\sqrt{2}\,\text{Cos}[t]^4\sqrt{3+\text{Cos}[2\,t]}$$

$$\text{Sin}[t]\Big)\Big/\left(2\,\text{Cos}[t]^2+2\sqrt{2}\,\text{Cos}[t]\,\text{Sin}[t]+3\,\text{Sin}[t]^2\right)^3-$$

$$\left(432\sqrt{2}\,\text{Cos}[t]^2\,\text{Cos}[2\,t]\sqrt{3+\text{Cos}[2\,t]}\,\text{Sin}[t]\right)\Big/$$

$$\left(2\,\text{Cos}[t]^2+2\sqrt{2}\,\text{Cos}[t]\,\text{Sin}[t]+3\,\text{Sin}[t]^2\right)^3-$$

$$\left(1296\,\text{Sin}[t]^2\right)\Big/\left(2\,\text{Cos}[t]^2+2\sqrt{2}\,\text{Cos}[t]\,\text{Sin}[t]+3\,\text{Sin}[t]^2\right)^3+$$

```
(5184 Cos[t]^2 Sin[t]^2) / (2 Cos[t]^2 + 2 Sqrt[2] Cos[t] Sin[t] + 3 Sin[t]^2)^3 +
(576 Cos[t]^4 Sin[t]^2) / (2 Cos[t]^2 + 2 Sqrt[2] Cos[t] Sin[t] + 3 Sin[t]^2)^3 -
(864 Cos[2 t] Sin[t]^2) / (2 Cos[t]^2 + 2 Sqrt[2] Cos[t] Sin[t] + 3 Sin[t]^2)^3 +
(1728 Cos[t]^2 Cos[2 t] Sin[t]^2) / (2 Cos[t]^2 +
    2 Sqrt[2] Cos[t] Sin[t] + 3 Sin[t]^2)^3 - (144 Cos[2 t]^2 Sin[t]^2) /
  (2 Cos[t]^2 + 2 Sqrt[2] Cos[t] Sin[t] + 3 Sin[t]^2)^3 + (648 Sqrt[2] Sqrt[3 + Cos[2 t]]
   Sin[t]^3) / (2 Cos[t]^2 + 2 Sqrt[2] Cos[t] Sin[t] + 3 Sin[t]^2)^3 +
(864 Sqrt[2] Cos[t]^2 Sqrt[3 + Cos[2 t]] Sin[t]^3) / (2 Cos[t]^2 + 2 Sqrt[2] Cos[t]
     Sin[t] + 3 Sin[t]^2)^3 + (216 Sqrt[2] Cos[2 t] Sqrt[3 + Cos[2 t]] Sin[t]^3) /
  (2 Cos[t]^2 + 2 Sqrt[2] Cos[t] Sin[t] + 3 Sin[t]^2)^3 + (2160 Sin[t]^4) /
  (2 Cos[t]^2 + 2 Sqrt[2] Cos[t] Sin[t] + 3 Sin[t]^2)^3 - (1440 Cos[t]^2 Sin[t]^4) /
  (2 Cos[t]^2 + 2 Sqrt[2] Cos[t] Sin[t] + 3 Sin[t]^2)^3 + (720 Cos[2 t] Sin[t]^4) /
  (2 Cos[t]^2 + 2 Sqrt[2] Cos[t] Sin[t] + 3 Sin[t]^2)^3 - (864 Sqrt[2] Sqrt[3 + Cos[2 t]]
   Sin[t]^5) / (2 Cos[t]^2 + 2 Sqrt[2] Cos[t] Sin[t] + 3 Sin[t]^2)^3 +
(432 Sin[t]^6) / (2 Cos[t]^2 + 2 Sqrt[2] Cos[t] Sin[t] + 3 Sin[t]^2)^3)^2))^(1/3)))
```

The problem can only come from the expression under the square root, namely

```
badterm =
 FullSimplify[((4 (-9 - 24 Cos[t]^2 + 32 Cos[t]^4 - 6 Cos[2 t] - 8 Cos[t]^2 Cos[2 t] - Cos[2 t]^2 -
          72 Sin[t]^2 - 48 Cos[t]^2 Sin[t]^2 - 24 Cos[2 t] Sin[t]^2 + 12 Sin[t]^4)^3) /
     (2 Cos[t]^2 + 2 Sqrt[2] Cos[t] Sin[t] + 3 Sin[t]^2)^6 +
    (54 / (2 Cos[t]^2 + 2 Sqrt[2] Cos[t] Sin[t] + 3 Sin[t]^2)^3 +
      216 Cos[t]^2 / (2 Cos[t]^2 + 2 Sqrt[2] Cos[t] Sin[t] + 3 Sin[t]^2)^3 -
      1440 Cos[t]^4 / (2 Cos[t]^2 + 2 Sqrt[2] Cos[t] Sin[t] + 3 Sin[t]^2)^3 +
      1280 Cos[t]^6 / (2 Cos[t]^2 + 2 Sqrt[2] Cos[t] Sin[t] + 3 Sin[t]^2)^3 +
      54 Cos[2 t] / (2 Cos[t]^2 + 2 Sqrt[2] Cos[t] Sin[t] + 3 Sin[t]^2)^3 +
```

$$\frac{144\,\text{Cos}[t]^2\,\text{Cos}[2\,t]}{\left(2\,\text{Cos}[t]^2+2\sqrt{2}\,\text{Cos}[t]\,\text{Sin}[t]+3\,\text{Sin}[t]^2\right)^3}-$$

$$\frac{480\,\text{Cos}[t]^4\,\text{Cos}[2\,t]}{\left(2\,\text{Cos}[t]^2+2\sqrt{2}\,\text{Cos}[t]\,\text{Sin}[t]+3\,\text{Sin}[t]^2\right)^3}+$$

$$\frac{18\,\text{Cos}[2\,t]^2}{\left(2\,\text{Cos}[t]^2+2\sqrt{2}\,\text{Cos}[t]\,\text{Sin}[t]+3\,\text{Sin}[t]^2\right)^3}+$$

$$\frac{24\,\text{Cos}[t]^2\,\text{Cos}[2\,t]^2}{\left(2\,\text{Cos}[t]^2+2\sqrt{2}\,\text{Cos}[t]\,\text{Sin}[t]+3\,\text{Sin}[t]^2\right)^3}+$$

$$\frac{2\,\text{Cos}[2\,t]^3}{\left(2\,\text{Cos}[t]^2+2\sqrt{2}\,\text{Cos}[t]\,\text{Sin}[t]+3\,\text{Sin}[t]^2\right)^3}-$$

$$\frac{1296\sqrt{2}\,\text{Cos}[t]^2\sqrt{3+\text{Cos}[2\,t]}\,\text{Sin}[t]}{\left(2\,\text{Cos}[t]^2+2\sqrt{2}\,\text{Cos}[t]\,\text{Sin}[t]+3\,\text{Sin}[t]^2\right)^3}+$$

$$\frac{1728\sqrt{2}\,\text{Cos}[t]^4\sqrt{3+\text{Cos}[2\,t]}\,\text{Sin}[t]}{\left(2\,\text{Cos}[t]^2+2\sqrt{2}\,\text{Cos}[t]\,\text{Sin}[t]+3\,\text{Sin}[t]^2\right)^3}-$$

$$\frac{432\sqrt{2}\,\text{Cos}[t]^2\,\text{Cos}[2\,t]\sqrt{3+\text{Cos}[2\,t]}\,\text{Sin}[t]}{\left(2\,\text{Cos}[t]^2+2\sqrt{2}\,\text{Cos}[t]\,\text{Sin}[t]+3\,\text{Sin}[t]^2\right)^3}-$$

$$\frac{1296\,\text{Sin}[t]^2}{\left(2\,\text{Cos}[t]^2+2\sqrt{2}\,\text{Cos}[t]\,\text{Sin}[t]+3\,\text{Sin}[t]^2\right)^3}+$$

$$\frac{5184\,\text{Cos}[t]^2\,\text{Sin}[t]^2}{\left(2\,\text{Cos}[t]^2+2\sqrt{2}\,\text{Cos}[t]\,\text{Sin}[t]+3\,\text{Sin}[t]^2\right)^3}+$$

$$\frac{576\,\text{Cos}[t]^4\,\text{Sin}[t]^2}{\left(2\,\text{Cos}[t]^2+2\sqrt{2}\,\text{Cos}[t]\,\text{Sin}[t]+3\,\text{Sin}[t]^2\right)^3}-$$

$$\frac{864\,\text{Cos}[2\,t]\,\text{Sin}[t]^2}{\left(2\,\text{Cos}[t]^2+2\sqrt{2}\,\text{Cos}[t]\,\text{Sin}[t]+3\,\text{Sin}[t]^2\right)^3}+$$

$$\frac{1728\,\text{Cos}[t]^2\,\text{Cos}[2\,t]\,\text{Sin}[t]^2}{\left(2\,\text{Cos}[t]^2+2\sqrt{2}\,\text{Cos}[t]\,\text{Sin}[t]+3\,\text{Sin}[t]^2\right)^3}-$$

$$\frac{144\,\text{Cos}[2\,t]^2\,\text{Sin}[t]^2}{\left(2\,\text{Cos}[t]^2+2\sqrt{2}\,\text{Cos}[t]\,\text{Sin}[t]+3\,\text{Sin}[t]^2\right)^3}+$$

$$\frac{648\sqrt{2}\sqrt{3+\text{Cos}[2\,t]}\,\text{Sin}[t]^3}{\left(2\,\text{Cos}[t]^2+2\sqrt{2}\,\text{Cos}[t]\,\text{Sin}[t]+3\,\text{Sin}[t]^2\right)^3}+$$

$$\frac{864\sqrt{2}\,\text{Cos}[t]^2\sqrt{3+\text{Cos}[2\,t]}\,\text{Sin}[t]^3}{\left(2\,\text{Cos}[t]^2+2\sqrt{2}\,\text{Cos}[t]\,\text{Sin}[t]+3\,\text{Sin}[t]^2\right)^3}+$$

$$\frac{216\sqrt{2}\,\text{Cos}[2\,t]\sqrt{3+\text{Cos}[2\,t]}\,\text{Sin}[t]^3}{\left(2\,\text{Cos}[t]^2+2\sqrt{2}\,\text{Cos}[t]\,\text{Sin}[t]+3\,\text{Sin}[t]^2\right)^3}+$$

$$\frac{2160\,\text{Sin}[t]^4}{\left(2\,\text{Cos}[t]^2+2\sqrt{2}\,\text{Cos}[t]\,\text{Sin}[t]+3\,\text{Sin}[t]^2\right)^3}-$$
$$\frac{1440\,\text{Cos}[t]^2\,\text{Sin}[t]^4}{\left(2\,\text{Cos}[t]^2+2\sqrt{2}\,\text{Cos}[t]\,\text{Sin}[t]+3\,\text{Sin}[t]^2\right)^3}+$$
$$\frac{720\,\text{Cos}[2\,t]\,\text{Sin}[t]^4}{\left(2\,\text{Cos}[t]^2+2\sqrt{2}\,\text{Cos}[t]\,\text{Sin}[t]+3\,\text{Sin}[t]^2\right)^3}-$$
$$\frac{864\sqrt{2}\,\sqrt{3+\text{Cos}[2\,t]}\,\text{Sin}[t]^5}{\left(2\,\text{Cos}[t]^2+2\sqrt{2}\,\text{Cos}[t]\,\text{Sin}[t]+3\,\text{Sin}[t]^2\right)^3}+$$
$$\left.\left.\frac{432\,\text{Sin}[t]^6}{\left(2\,\text{Cos}[t]^2+2\sqrt{2}\,\text{Cos}[t]\,\text{Sin}[t]+3\,\text{Sin}[t]^2\right)^3}\right)^2\right)\Big]$$

$$-\Big(\Big(3456\,\text{Sin}[t]^2\,\Big(22\,830\,\text{Cos}[2\,t]+6392\,\text{Cos}[4\,t]+13\,595\,\text{Cos}[6\,t]+3170\,\text{Cos}[8\,t]+439\,\text{Cos}[10\,t]+2\,\Big(-6829+4\sqrt{2}\,\sqrt{3+\text{Cos}[2\,t]}\,\Big(845\,\text{Sin}[t]-1437\,\text{Sin}[3\,t]+423\,\text{Sin}[5\,t]+162\,\text{Sin}[7\,t]+81\,\text{Sin}[9\,t]\Big)\Big)\Big)\Big)\Big/\Big(-5+\text{Cos}[2\,t]-2\sqrt{2}\,\text{Sin}[2\,t]\Big)^6\Big)$$

So now we solve for when this expression vanishes.

```
Solve[badterm == 0 && 0 < t < 1/2, t, Reals]
```

```
{{t →
  2 ArcTan[Root[16 - 992 #1^2 + 9689 #1^4 - 36 232 #1^6 + 100 908 #1^8 - 197 080 #1^10 + 238 166 #1^12 -
      197 080 #1^14 + 100 908 #1^16 - 36 232 #1^18 + 9689 #1^20 - 992 #1^22 + 16 #1^24 &, 7]]}}
```

So, as claimed in the paper, the correct value of $t$ is $t_0 = 2\arctan(\alpha)$, where $\alpha$ is the seventh root of the polynomial

```
16 - 992 #1^2 + 9689 #1^4 - 36 232 #1^6 + 100 908 #1^8 - 197 080 #1^10 + 238 166 #1^12 -
  197 080 #1^14 + 100 908 #1^16 - 36 232 #1^18 + 9689 #1^20 - 992 #1^22 + 16 #1^24 &[z]
```

$$16-992\,z^2+9689\,z^4-36\,232\,z^6+100\,908\,z^8-197\,080\,z^{10}+238\,166\,z^{12}-197\,080\,z^{14}+100\,908\,z^{16}-36\,232\,z^{18}+9689\,z^{20}-992\,z^{22}+16\,z^{24}$$

and we see that the seventh root is the smallest positive root:

```
TableForm@Table[{i, N[
    Root[16 - 992 #1^2 + 9689 #1^4 - 36 232 #1^6 + 100 908 #1^8 - 197 080 #1^10 + 238 166 #1^12 - 197 080
       #1^14 + 100 908 #1^16 - 36 232 #1^18 + 9689 #1^20 - 992 #1^22 + 16 #1^24 &, i]]}, {i, 1, 24}]
```

| | |
|---|---|
| 1 | -7.13714 |
| 2 | -2.61199 |
| 3 | -1.35783 |
| 4 | -0.736468 |
| 5 | -0.38285 |
| 6 | -0.140112 |
| 7 | 0.140112 |
| 8 | 0.38285 |
| 9 | 0.736468 |
| 10 | 1.35783 |
| 11 | 2.61199 |
| 12 | 7.13714 |
| 13 | -1.1465 - 1.02639 i |
| 14 | -1.1465 + 1.02639 i |
| 15 | -0.876274 - 0.481812 i |
| 16 | -0.876274 + 0.481812 i |
| 17 | -0.484174 - 0.433454 i |
| 18 | -0.484174 + 0.433454 i |
| 19 | 0.484174 - 0.433454 i |
| 20 | 0.484174 + 0.433454 i |
| 21 | 0.876274 - 0.481812 i |
| 22 | 0.876274 + 0.481812 i |
| 23 | 1.1465 - 1.02639 i |
| 24 | 1.1465 + 1.02639 i |

# Most scalene acute triangle

The same strategy works for finding the most scalene acute triangle. The points of interest are those on the curve

$$\tilde{p}(t) = \cos(t)\left(\frac{1}{\sqrt{3}}, \frac{1}{\sqrt{3}}, \frac{1}{\sqrt{3}}\right) + \sin(t)\left(\frac{1}{\sqrt{2}}, 0, -\frac{1}{\sqrt{2}}\right)$$

```
p2[t_] := Cos[t] 1/Sqrt[3] {1, 1, 1} + Sin[t] 1/Sqrt[2] {1, 0, -1};
```

and the distance from $\tilde{p}(t)$ to $q(x)$ is

```
ArcCos[p2[t].q[x]]
```

$$\mathrm{ArcCos}\left[\frac{\sqrt{\frac{1-x^2}{1+x^2}}\ \mathrm{Cos}[t]}{\sqrt{3}} + x\sqrt{\frac{1-x^2}{1+x^2}}\left(\frac{\mathrm{Cos}[t]}{\sqrt{3}} - \frac{\mathrm{Sin}[t]}{\sqrt{2}}\right) + x\left(\frac{\mathrm{Cos}[t]}{\sqrt{3}} + \frac{\mathrm{Sin}[t]}{\sqrt{2}}\right)\right]$$

whereas the distance from $\tilde{p}(t)$ to either of the bounding great circles is $\arcsin\left(\frac{\sin(t)}{2}\right)$. So we solve for those values of $x$ for which these two distances are equal:

sols2 =

$$\text{Solve}\left[\text{ArcCos}\left[\frac{\sqrt{\frac{1-x^2}{1+x^2}}\ \text{Cos}[t]}{\sqrt{3}} + x\sqrt{\frac{1-x^2}{1+x^2}}\left(\frac{\text{Cos}[t]}{\sqrt{3}} - \frac{\text{Sin}[t]}{\sqrt{2}}\right) + x\left(\frac{\text{Cos}[t]}{\sqrt{3}} + \frac{\text{Sin}[t]}{\sqrt{2}}\right)\right] == \text{ArcSin}[\text{Sin}[t]/2], x\right]$$

$$\Bigg\{\Bigg\{x \to -\Bigg(\Bigg(2\,\text{Cos}[t]^2 - \sqrt{6}\ \text{Cos}[t]\ \text{Sin}[t] - 2\sqrt{3}\ \text{Cos}[t]\ \sqrt{1 - \frac{\langle\langle 1 \rangle\rangle^2}{4}} - 3\sqrt{2}\ \text{Sin}[t]\ \sqrt{1 - \frac{\text{Sin}[t]^2}{4}}\Bigg)\Big/\left(4\left(2\,\text{Cos}[t]^2 + 3\,\text{Sin}[t]^2\right)\right)\Bigg) -$$

$$\frac{1}{2}\sqrt{\left(\frac{\text{Cos}[t]^4}{\left(\langle\langle 1 \rangle\rangle\right)^2} - \frac{\sqrt{6}\ \langle\langle 1 \rangle\rangle^3\ \text{Sin}[t]}{\left(\langle\langle 1 \rangle\rangle\right)^2} + \langle\langle 23 \rangle\rangle + \frac{\langle\langle 1 \rangle\rangle}{\langle\langle 1 \rangle\rangle} + \frac{\left(\langle\langle 1 \rangle\rangle\right)^{1/3}}{3 \times 2^{1/3}}\right)} -$$

$$\frac{1}{2}\sqrt{-\frac{\text{Cos}[t]^4}{\left(2\ \langle\langle 1 \rangle\rangle^2 + \langle\langle 1 \rangle\rangle\right)^2} + \langle\langle 35 \rangle\rangle}\Bigg\},$$

$$\{x \to \langle\langle 1 \rangle\rangle\},\ \langle\langle 1 \rangle\rangle,\ \{x \to \langle\langle 1 \rangle\rangle\}\Bigg\}$$

large output | **show less** | **show more** | **show all** | **set size limit...**

Again, we're looking for the smallest value of *t* that yields a real solution

```
Plot[Evaluate[x /. # & /@ sols2], {t, 0, π/8}]
```

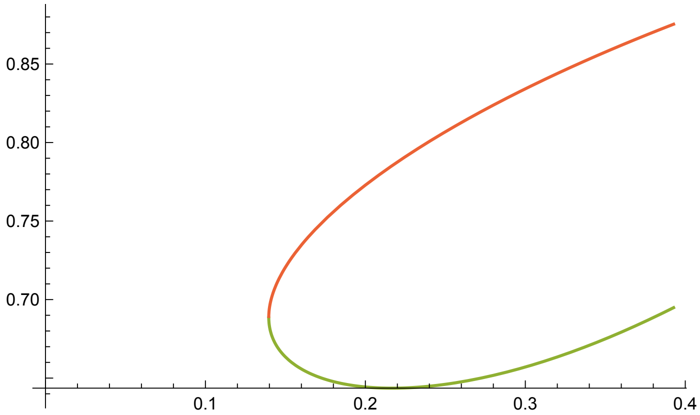


...which is now slightly larger than 0.1. Again, the third and fourth solutions switch from complex to real at this point, so we focus on the third solution.

```
x /. sols2[[3]]
```

$$-\left(\left(\left(2\,\mathrm{Cos}[t]^2-\sqrt{6}\,\mathrm{Cos}[t]\,\mathrm{Sin}[t]-2\sqrt{3}\,\mathrm{Cos}[t]\sqrt{1-\frac{\cdots 1\cdots^2}{4}}-3\sqrt{2}\,\mathrm{Sin}[t]\sqrt{1-\frac{\mathrm{Sin}[t]^2}{4}}\right)\Big/\left(4\left(2\,\mathrm{Cos}[t]^2+3\,\mathrm{Sin}[t]^2\right)\right)\right)+\frac{1}{2}\sqrt{\cdots 27\cdots+\frac{\cdots 1\cdots^{\cdots 1\cdots}}{3\times 2^{\cdots 1\cdots}}}-\frac{1}{2}\sqrt{\left(-\frac{\mathrm{Cos}[t]^4}{\left(2\,\cdots 1\cdots^2+3\,\cdots 1\cdots\right)^2}+\cdots 33\cdots+\frac{-\frac{8\left(\cdots 1\cdots\right)}{2\,\cdots 1\cdots+\cdots 1\cdots}+\cdots 1\cdots}{4\sqrt{\cdots 1\cdots}}\right)}$$

large output | show less | show more | show all | set size limit...

Just as before, the trouble is under the last square root:

```
complexterm2 = %[[3, 2, 1]]
```

$$-\frac{\mathrm{Cos}[t]^4}{\left(2\,\mathrm{Cos}[t]^2+3\,\mathrm{Sin}[t]^2\right)^2}+\cdots 33\cdots+\frac{-\frac{8\left(-2\,\cdots 1\cdots^2+\cdots 5\cdots\right)}{2\,\mathrm{Cos}[t]^2+3\,\cdots 1\cdots^2}+\frac{\left(\cdots 1\cdots\right)\,\cdots 1\cdots}{2\,\cdots 1\cdots+\cdots 1\cdots}}{4\sqrt{\frac{\mathrm{Cos}[t]^4}{\left(\cdots 1\cdots\right)^2}-\frac{\sqrt{6}\,\cdots 1\cdots^3\,\mathrm{Sin}[t]}{\left(\cdots 1\cdots\right)^2}+\cdots 23\cdots+\frac{\cdots 1\cdots}{\cdots 1\cdots}+\frac{\left(\cdots 1\cdots\right)^{1/3}}{3\times 2^{1/3}}}}$$

large output | show less | show more | show all | set size limit...

and some terms are real and some aren’t:

```
TableForm@Table[{i, complexterm2[[i]] /. t → .1}, {i, 1, Length[complexterm2]}]
```

| | |
|---|---|
| 1 | -0.242617 |
| 2 | 0.0596278 |
| 3 | -0.00366366 |
| 4 | 0.843618 |
| 5 | -0.0127391 |
| 6 | -0.733348 |
| 7 | -0.180234 |
| 8 | -0.011074 |
| 9 | 0.328375 |
| 10 | -0.0807042 |
| 11 | 0.242113 |
| 12 | 0.992562 |
| 13 | 0.841289 |
| 14 | -4.44704 |
| 15 | 0.311916 - 0.0331295 i |
| 16 | 0.0557522 - 0.00592159 i |
| 17 | -0.00171277 + 0.000181918 i |
| 18 | -1.19995 + 0.127449 i |
| 19 | 0.168519 - 0.0178989 i |
| 20 | -0.0155313 + 0.00164962 i |
| 21 | -0.259073 + 0.0275168 i |
| 22 | -0.940074 - 0.0998478 i |
| 23 | $4.26999 + 6.55285\times 10^{-17}$ i |

Again, the complex terms become real at the same moment the expression changes from negative to positive; since this expression is under a square root, this is when the whole expression changes from complex to real.

```
Plot[
 Evaluate@Prepend[Table[complexterm2[[i]], {i, 15, 22}], complexterm2], {t, 0, π/8}]
```

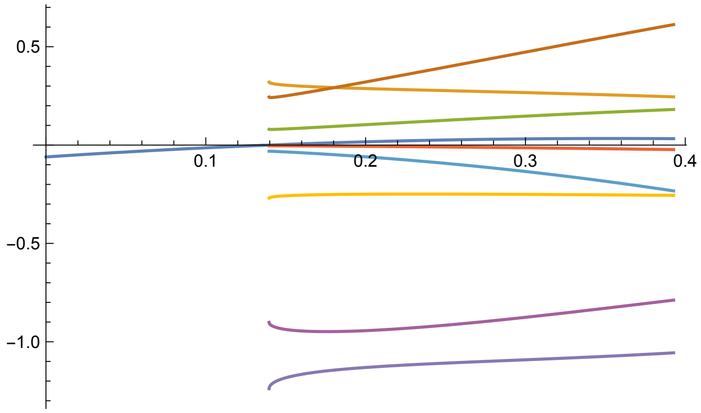


Again, the trouble is the expression under the square root in any of these terms:

```
complexterm2[[15]]
```

$$
\begin{aligned}
&\left(11 \times 2^{1/3}\,\mathrm{Cos}[t]^4\right) \Big/ \\
&\Bigg(3\,\left(2\,\mathrm{Cos}[t]^2+3\,\mathrm{Sin}[t]^2\right)^2 \Bigg(\frac{290\,\mathrm{Cos}[t]^6}{\left(2\,\mathrm{Cos}[t]^2+3\,\mathrm{Sin}[t]^2\right)^3}+\frac{228\sqrt{6}\,\mathrm{Cos}[t]^5\,\mathrm{Sin}[t]}{\left(2\,\mathrm{Cos}[t]^2+3\,\mathrm{Sin}[t]^2\right)^3}+ \\
&\frac{468\,\mathrm{Cos}[t]^4\,\mathrm{Sin}[t]^2}{\left(2\,\mathrm{Cos}[t]^2+3\,\mathrm{Sin}[t]^2\right)^3}+\frac{312\sqrt{6}\,\mathrm{Cos}[t]^3\,\mathrm{Sin}[t]^3}{\left(2\,\mathrm{Cos}[t]^2+3\,\mathrm{Sin}[t]^2\right)^3}+\frac{486\,\mathrm{Cos}[t]^2\,\mathrm{Sin}[t]^4}{\left(2\,\mathrm{Cos}[t]^2+3\,\mathrm{Sin}[t]^2\right)^3}+ \\
&\frac{648\sqrt{3}\,\mathrm{Cos}[t]^5\sqrt{1-\frac{\mathrm{Sin}[t]^2}{4}}}{\left(2\,\mathrm{Cos}[t]^2+3\,\mathrm{Sin}[t]^2\right)^3}-\frac{324\sqrt{3}\,\mathrm{Cos}[t]^3\,\mathrm{Sin}[t]^2\sqrt{1-\frac{\mathrm{Sin}[t]^2}{4}}}{\left(2\,\mathrm{Cos}[t]^2+3\,\mathrm{Sin}[t]^2\right)^3}- \\
&\frac{972\sqrt{3}\,\mathrm{Cos}[t]\,\mathrm{Sin}[t]^4\sqrt{1-\frac{\mathrm{Sin}[t]^2}{4}}}{\left(2\,\mathrm{Cos}[t]^2+3\,\mathrm{Sin}[t]^2\right)^3}+\frac{666\,\mathrm{Cos}[t]^4\left(1-\frac{\mathrm{Sin}[t]^2}{4}\right)}{\left(2\,\mathrm{Cos}[t]^2+3\,\mathrm{Sin}[t]^2\right)^3}- \\
&\frac{1224\sqrt{6}\,\mathrm{Cos}[t]^3\,\mathrm{Sin}[t]\left(1-\frac{\mathrm{Sin}[t]^2}{4}\right)}{\left(2\,\mathrm{Cos}[t]^2+3\,\mathrm{Sin}[t]^2\right)^3}+\frac{1080\,\mathrm{Cos}[t]^2\,\mathrm{Sin}[t]^2\left(1-\frac{\mathrm{Sin}[t]^2}{4}\right)}{\left(2\,\mathrm{Cos}[t]^2+3\,\mathrm{Sin}[t]^2\right)^3}- \\
&\frac{648\sqrt{6}\,\mathrm{Cos}[t]\,\mathrm{Sin}[t]^3\left(1-\frac{\mathrm{Sin}[t]^2}{4}\right)}{\left(2\,\mathrm{Cos}[t]^2+3\,\mathrm{Sin}[t]^2\right)^3}+\frac{1458\,\mathrm{Sin}[t]^4\left(1-\frac{\mathrm{Sin}[t]^2}{4}\right)}{\left(2\,\mathrm{Cos}[t]^2+3\,\mathrm{Sin}[t]^2\right)^3}- \\
&\frac{648\sqrt{3}\,\mathrm{Cos}[t]^3\left(1-\frac{\mathrm{Sin}[t]^2}{4}\right)^{3/2}}{\left(2\,\mathrm{Cos}[t]^2+3\,\mathrm{Sin}[t]^2\right)^3}+\frac{972\sqrt{3}\,\mathrm{Cos}[t]\,\mathrm{Sin}[t]^2\left(1-\frac{\mathrm{Sin}[t]^2}{4}\right)^{3/2}}{\left(2\,\mathrm{Cos}[t]^2+3\,\mathrm{Sin}[t]^2\right)^3}- \\
&\frac{594\,\mathrm{Cos}[t]^2\left(1-\frac{\mathrm{Sin}[t]^2}{4}\right)^2}{\left(2\,\mathrm{Cos}[t]^2+3\,\mathrm{Sin}[t]^2\right)^3}+\frac{756\sqrt{6}\,\mathrm{Cos}[t]\,\mathrm{Sin}[t]\left(1-\frac{\mathrm{Sin}[t]^2}{4}\right)^2}{\left(2\,\mathrm{Cos}[t]^2+3\,\mathrm{Sin}[t]^2\right)^3}- \\
&\frac{972\,\mathrm{Sin}[t]^2\left(1-\frac{\mathrm{Sin}[t]^2}{4}\right)^2}{\left(2\,\mathrm{Cos}[t]^2+3\,\mathrm{Sin}[t]^2\right)^3}+\frac{54\left(1-\frac{\mathrm{Sin}[t]^2}{4}\right)^3}{\left(2\,\mathrm{Cos}[t]^2+3\,\mathrm{Sin}[t]^2\right)^3}+
\end{aligned}
$$

$$
\sqrt{\left(\left(\frac{4\left(11\,\text{Cos}[t]^4+8\sqrt{6}\,\text{Cos}[t]^3\,\text{Sin}[t]-6\,\text{Cos}[t]^2\,\text{Sin}[t]^2-42\,\text{Cos}[t]^2\left(1-\frac{\text{Sin}[t]^2}{4}\right)+24\sqrt{6}\,\text{Cos}[t]\,\text{Sin}[t]\left(1-\frac{\text{Sin}[t]^2}{4}\right)-54\,\text{Sin}[t]^2\left(1-\frac{\text{Sin}[t]^2}{4}\right)-9\left(1-\frac{\text{Sin}[t]^2}{4}\right)^2\right)^3}{\left(2\,\text{Cos}[t]^2+3\,\text{Sin}[t]^2\right)^6}+\left(\frac{290\,\text{Cos}[t]^6}{\left(2\,\text{Cos}[t]^2+3\,\text{Sin}[t]^2\right)^3}+\frac{228\sqrt{6}\,\text{Cos}[t]^5\,\text{Sin}[t]}{\left(2\,\text{Cos}[t]^2+3\,\text{Sin}[t]^2\right)^3}+\frac{468\,\text{Cos}[t]^4\,\text{Sin}[t]^2}{\left(2\,\text{Cos}[t]^2+3\,\text{Sin}[t]^2\right)^3}+\frac{312\sqrt{6}\,\text{Cos}[t]^3\,\text{Sin}[t]^3}{\left(2\,\text{Cos}[t]^2+3\,\text{Sin}[t]^2\right)^3}+\frac{486\,\text{Cos}[t]^2\,\text{Sin}[t]^4}{\left(2\,\text{Cos}[t]^2+3\,\text{Sin}[t]^2\right)^3}+\frac{648\sqrt{3}\,\text{Cos}[t]^5\sqrt{1-\frac{\text{Sin}[t]^2}{4}}}{\left(2\,\text{Cos}[t]^2+3\,\text{Sin}[t]^2\right)^3}-\frac{324\sqrt{3}\,\text{Cos}[t]^3\,\text{Sin}[t]^2\sqrt{1-\frac{\text{Sin}[t]^2}{4}}}{\left(2\,\text{Cos}[t]^2+3\,\text{Sin}[t]^2\right)^3}-\frac{972\sqrt{3}\,\text{Cos}[t]\,\text{Sin}[t]^4\sqrt{1-\frac{\text{Sin}[t]^2}{4}}}{\left(2\,\text{Cos}[t]^2+3\,\text{Sin}[t]^2\right)^3}+\frac{666\,\text{Cos}[t]^4\left(1-\frac{\text{Sin}[t]^2}{4}\right)}{\left(2\,\text{Cos}[t]^2+3\,\text{Sin}[t]^2\right)^3}-\frac{1224\sqrt{6}\,\text{Cos}[t]^3\,\text{Sin}[t]\left(1-\frac{\text{Sin}[t]^2}{4}\right)}{\left(2\,\text{Cos}[t]^2+3\,\text{Sin}[t]^2\right)^3}+\frac{1080\,\text{Cos}[t]^2\,\text{Sin}[t]^2\left(1-\frac{\text{Sin}[t]^2}{4}\right)}{\left(2\,\text{Cos}[t]^2+3\,\text{Sin}[t]^2\right)^3}-\frac{648\sqrt{6}\,\text{Cos}[t]\,\text{Sin}[t]^3\left(1-\frac{\text{Sin}[t]^2}{4}\right)}{\left(2\,\text{Cos}[t]^2+3\,\text{Sin}[t]^2\right)^3}+\frac{1458\,\text{Sin}[t]^4\left(1-\frac{\text{Sin}[t]^2}{4}\right)}{\left(2\,\text{Cos}[t]^2+3\,\text{Sin}[t]^2\right)^3}-\frac{648\sqrt{3}\,\text{Cos}[t]^3\left(1-\frac{\text{Sin}[t]^2}{4}\right)^{3/2}}{\left(2\,\text{Cos}[t]^2+3\,\text{Sin}[t]^2\right)^3}+\frac{972\sqrt{3}\,\text{Cos}[t]\,\text{Sin}[t]^2\left(1-\frac{\text{Sin}[t]^2}{4}\right)^{3/2}}{\left(2\,\text{Cos}[t]^2+3\,\text{Sin}[t]^2\right)^3}-\frac{594\,\text{Cos}[t]^2\left(1-\frac{\text{Sin}[t]^2}{4}\right)^2}{\left(2\,\text{Cos}[t]^2+3\,\text{Sin}[t]^2\right)^3}+\frac{756\sqrt{6}\,\text{Cos}[t]\,\text{Sin}[t]\left(1-\frac{\text{Sin}[t]^2}{4}\right)^2}{\left(2\,\text{Cos}[t]^2+3\,\text{Sin}[t]^2\right)^3}-\frac{972\,\text{Sin}[t]^2\left(1-\frac{\text{Sin}[t]^2}{4}\right)^2}{\left(2\,\text{Cos}[t]^2+3\,\text{Sin}[t]^2\right)^3}+\frac{54\left(1-\frac{\text{Sin}[t]^2}{4}\right)^3}{\left(2\,\text{Cos}[t]^2+3\,\text{Sin}[t]^2\right)^3}\right)^2\right)^{1/3}\right)}
$$

$$
\begin{aligned}
&\text{badterm2} = \text{FullSimplify}\Bigg[\\
&\Bigg(\Bigg(4\,\Bigg(11\,\text{Cos}[t]^4 + 8\sqrt{6}\,\text{Cos}[t]^3\,\text{Sin}[t] - 6\,\text{Cos}[t]^2\,\text{Sin}[t]^2 - 42\,\text{Cos}[t]^2\left(1-\frac{\text{Sin}[t]^2}{4}\right) +\\
&\qquad 24\sqrt{6}\,\text{Cos}[t]\,\text{Sin}[t]\left(1-\frac{\text{Sin}[t]^2}{4}\right) - 54\,\text{Sin}[t]^2\left(1-\frac{\text{Sin}[t]^2}{4}\right) -\\
&\qquad 9\left(1-\frac{\text{Sin}[t]^2}{4}\right)^2\Bigg)^3\Bigg) \Big/ \left(2\,\text{Cos}[t]^2 + 3\,\text{Sin}[t]^2\right)^6 +\\
&\Bigg(\frac{290\,\text{Cos}[t]^6}{\left(2\,\text{Cos}[t]^2 + 3\,\text{Sin}[t]^2\right)^3} + \frac{228\sqrt{6}\,\text{Cos}[t]^5\,\text{Sin}[t]}{\left(2\,\text{Cos}[t]^2 + 3\,\text{Sin}[t]^2\right)^3} + \frac{468\,\text{Cos}[t]^4\,\text{Sin}[t]^2}{\left(2\,\text{Cos}[t]^2 + 3\,\text{Sin}[t]^2\right)^3} +\\
&\qquad \frac{312\sqrt{6}\,\text{Cos}[t]^3\,\text{Sin}[t]^3}{\left(2\,\text{Cos}[t]^2 + 3\,\text{Sin}[t]^2\right)^3} + \frac{486\,\text{Cos}[t]^2\,\text{Sin}[t]^4}{\left(2\,\text{Cos}[t]^2 + 3\,\text{Sin}[t]^2\right)^3} +\\
&\qquad \frac{648\sqrt{3}\,\text{Cos}[t]^5\sqrt{1-\frac{\text{Sin}[t]^2}{4}}}{\left(2\,\text{Cos}[t]^2 + 3\,\text{Sin}[t]^2\right)^3} - \frac{324\sqrt{3}\,\text{Cos}[t]^3\,\text{Sin}[t]^2\sqrt{1-\frac{\text{Sin}[t]^2}{4}}}{\left(2\,\text{Cos}[t]^2 + 3\,\text{Sin}[t]^2\right)^3} -\\
&\qquad \frac{972\sqrt{3}\,\text{Cos}[t]\,\text{Sin}[t]^4\sqrt{1-\frac{\text{Sin}[t]^2}{4}}}{\left(2\,\text{Cos}[t]^2 + 3\,\text{Sin}[t]^2\right)^3} + \frac{666\,\text{Cos}[t]^4\left(1-\frac{\text{Sin}[t]^2}{4}\right)}{\left(2\,\text{Cos}[t]^2 + 3\,\text{Sin}[t]^2\right)^3} -\\
&\qquad \frac{1224\sqrt{6}\,\text{Cos}[t]^3\,\text{Sin}[t]\left(1-\frac{\text{Sin}[t]^2}{4}\right)}{\left(2\,\text{Cos}[t]^2 + 3\,\text{Sin}[t]^2\right)^3} + \frac{1080\,\text{Cos}[t]^2\,\text{Sin}[t]^2\left(1-\frac{\text{Sin}[t]^2}{4}\right)}{\left(2\,\text{Cos}[t]^2 + 3\,\text{Sin}[t]^2\right)^3} -\\
&\qquad \frac{648\sqrt{6}\,\text{Cos}[t]\,\text{Sin}[t]^3\left(1-\frac{\text{Sin}[t]^2}{4}\right)}{\left(2\,\text{Cos}[t]^2 + 3\,\text{Sin}[t]^2\right)^3} + \frac{1458\,\text{Sin}[t]^4\left(1-\frac{\text{Sin}[t]^2}{4}\right)}{\left(2\,\text{Cos}[t]^2 + 3\,\text{Sin}[t]^2\right)^3} -\\
&\qquad \frac{648\sqrt{3}\,\text{Cos}[t]^3\left(1-\frac{\text{Sin}[t]^2}{4}\right)^{3/2}}{\left(2\,\text{Cos}[t]^2 + 3\,\text{Sin}[t]^2\right)^3} + \frac{972\sqrt{3}\,\text{Cos}[t]\,\text{Sin}[t]^2\left(1-\frac{\text{Sin}[t]^2}{4}\right)^{3/2}}{\left(2\,\text{Cos}[t]^2 + 3\,\text{Sin}[t]^2\right)^3} -\\
&\qquad \frac{594\,\text{Cos}[t]^2\left(1-\frac{\text{Sin}[t]^2}{4}\right)^2}{\left(2\,\text{Cos}[t]^2 + 3\,\text{Sin}[t]^2\right)^3} + \frac{756\sqrt{6}\,\text{Cos}[t]\,\text{Sin}[t]\left(1-\frac{\text{Sin}[t]^2}{4}\right)^2}{\left(2\,\text{Cos}[t]^2 + 3\,\text{Sin}[t]^2\right)^3} -\\
&\qquad \frac{972\,\text{Sin}[t]^2\left(1-\frac{\text{Sin}[t]^2}{4}\right)^2}{\left(2\,\text{Cos}[t]^2 + 3\,\text{Sin}[t]^2\right)^3} + \frac{54\left(1-\frac{\text{Sin}[t]^2}{4}\right)^3}{\left(2\,\text{Cos}[t]^2 + 3\,\text{Sin}[t]^2\right)^3}\Bigg)^2\Bigg)\Bigg]
\end{aligned}
$$

$$\frac{1}{16384\,\left(-5+\mathrm{Cos}[2\,t]\right)^6}\Big(2\,\left(-5787+356\,\mathrm{Cos}[2\,t]+311\,\mathrm{Cos}[4\,t]+1600\,\sqrt{6}\,\mathrm{Sin}[2\,t]+224\,\sqrt{6}\,\mathrm{Sin}[4\,t]\right)^3+\Big(402346-97599\,\mathrm{Cos}[2\,t]+102246\,\mathrm{Cos}[4\,t]+18991\,\mathrm{Cos}[6\,t]+5184\,\sqrt{6}\,\sqrt{7+\mathrm{Cos}[2\,t]}\,\left(3\,\mathrm{Cos}[t]+5\,\mathrm{Cos}[3\,t]\right)\mathrm{Sin}[t]^2-59640\,\sqrt{6}\,\mathrm{Sin}[2\,t]-22944\,\sqrt{6}\,\mathrm{Sin}[4\,t]-5784\,\sqrt{6}\,\mathrm{Sin}[6\,t]\Big)^2\Big)$$

Given sufficient time, *Mathematica* will find the desired root

```
TimeConstrained[Solve[badterm2 == 0 && 0 < t < 1 / 4, t, Reals], 3600]
```

```
{{t →
   2 ArcTan[Root[131 072 - 30 081 024 #1^2 + 715 784 192 #1^4 - 10 181 738 496 #1^6 + 83 609 604 096
          #1^8 - 443 259 328 512 #1^10 + 1 410 471 953 408 #1^12 - 1 858 643 071 488 #1^14 +
        18 137 673 285 920 #1^16 - 14 367 112 128 688 #1^18 + 56 162 265 469 488 #1^20 -
        73 041 229 883 512 #1^22 + 73 382 345 772 378 #1^24 - 122 601 623 733 111 #1^26 +
        73 382 345 772 378 #1^28 - 73 041 229 883 512 #1^30 + 56 162 265 469 488 #1^32 -
        14 367 112 128 688 #1^34 + 18 137 673 285 920 #1^36 - 1 858 643 071 488 #1^38 +
        1 410 471 953 408 #1^40 - 443 259 328 512 #1^42 + 83 609 604 096 #1^44 -
        10 181 738 496 #1^46 + 715 784 192 #1^48 - 30 081 024 #1^50 + 131 072 #1^52 &, 7]]}}
```

...namely, $\tilde{t}_0 = 2\arctan\tilde{\alpha}$, where $\tilde{\alpha}$ is the seventh root of the polynomial

```
131 072 - 30 081 024 #1^2 + 715 784 192 #1^4 - 10 181 738 496 #1^6 + 83 609 604 096 #1^8 -
    443 259 328 512 #1^10 + 1 410 471 953 408 #1^12 - 1 858 643 071 488 #1^14 +
    18 137 673 285 920 #1^16 - 14 367 112 128 688 #1^18 + 56 162 265 469 488 #1^20 -
    73 041 229 883 512 #1^22 + 73 382 345 772 378 #1^24 - 122 601 623 733 111 #1^26 +
    73 382 345 772 378 #1^28 - 73 041 229 883 512 #1^30 + 56 162 265 469 488 #1^32 -
    14 367 112 128 688 #1^34 + 18 137 673 285 920 #1^36 - 1 858 643 071 488 #1^38 +
    1 410 471 953 408 #1^40 - 443 259 328 512 #1^42 + 83 609 604 096 #1^44 -
    10 181 738 496 #1^46 + 715 784 192 #1^48 - 30 081 024 #1^50 + 131 072 #1^52 &[z]
```

$$131072-30081024\,z^{2}+715784192\,z^{4}-10181738496\,z^{6}+83609604096\,z^{8}-443259328512\,z^{10}+1410471953408\,z^{12}-1858643071488\,z^{14}+18137673285920\,z^{16}-14367112128688\,z^{18}+56162265469488\,z^{20}-73041229883512\,z^{22}+73382345772378\,z^{24}-122601623733111\,z^{26}+73382345772378\,z^{28}-73041229883512\,z^{30}+56162265469488\,z^{32}-14367112128688\,z^{34}+18137673285920\,z^{36}-1858643071488\,z^{38}+1410471953408\,z^{40}-443259328512\,z^{42}+83609604096\,z^{44}-10181738496\,z^{46}+715784192\,z^{48}-30081024\,z^{50}+131072\,z^{52}$$

We verify that the seventh root is indeed the smallest positive root:

```
TableForm@Table[
  {i, N[Root[131 072 - 30 081 024 #1^2 + 715 784 192 #1^4 - 10 181 738 496 #1^6 + 83 609 604 096 #1^8 -
        443 259 328 512 #1^10 + 1 410 471 953 408 #1^12 - 1 858 643 071 488 #1^14 +
        18 137 673 285 920 #1^16 - 14 367 112 128 688 #1^18 + 56 162 265 469 488 #1^20 -
        73 041 229 883 512 #1^22 + 73 382 345 772 378 #1^24 - 122 601 623 733 111 #1^26 +
        73 382 345 772 378 #1^28 - 73 041 229 883 512 #1^30 + 56 162 265 469 488 #1^32 -
        14 367 112 128 688 #1^34 + 18 137 673 285 920 #1^36 - 1 858 643 071 488 #1^38 +
        1 410 471 953 408 #1^40 - 443 259 328 512 #1^42 + 83 609 604 096 #1^44 - 10 181 738 496 #1^46 +
        715 784 192 #1^48 - 30 081 024 #1^50 + 131 072 #1^52 &, i]]}, {i, 1, 52}]
```

| | |
|---|---|
| 1 | -14.3035 |
| 2 | -2.84231 |
| 3 | -1.04403 |
| 4 | -0.957824 |
| 5 | -0.351827 |
| 6 | -0.0699128 |
| 7 | 0.0699128 |
| 8 | 0.351827 |
| 9 | 0.957824 |
| 10 | 1.04403 |
| 11 | 2.84231 |
| 12 | 14.3035 |
| 13 | -2.90065 - 1.45724 i |
| 14 | -2.90065 + 1.45724 i |
| 15 | -2.40338 - 1.59391 i |
| 16 | -2.40338 + 1.59391 i |
| 17 | -0.815224 - 1.4638 i |
| 18 | -0.815224 + 1.4638 i |
| 19 | -0.813385 - 0.925832 i |
| 20 | -0.813385 + 0.925832 i |
| 21 | -0.664394 - 0.787029 i |
| 22 | -0.664394 + 0.787029 i |
| 23 | -0.626294 - 0.741897 i |
| 24 | -0.626294 + 0.741897 i |
| 25 | -0.535559 - 0.609597 i |
| 26 | -0.535559 + 0.609597 i |
| 27 | -0.290393 - 0.521426 i |
| 28 | -0.290393 + 0.521426 i |
| 29 | -0.28898 - 0.19165 i |
| 30 | -0.28898 + 0.19165 i |
| 31 | -0.275274 - 0.138294 i |
| 32 | -0.275274 + 0.138294 i |
| 33 | 0.275274 - 0.138294 i |
| 34 | 0.275274 + 0.138294 i |
| 35 | 0.28898 - 0.19165 i |
| 36 | 0.28898 + 0.19165 i |
| 37 | 0.290393 - 0.521426 i |
| 38 | 0.290393 + 0.521426 i |
| 39 | 0.535559 - 0.609597 i |
| 40 | 0.535559 + 0.609597 i |
| 41 | 0.626294 - 0.741897 i |
| 42 | 0.626294 + 0.741897 i |
| 43 | 0.664394 - 0.787029 i |
| 44 | 0.664394 + 0.787029 i |
| 45 | 0.813385 - 0.925832 i |
| 46 | 0.813385 + 0.925832 i |
| 47 | 0.815224 - 1.4638 i |
| 48 | 0.815224 + 1.4638 i |
| 49 | 2.40338 - 1.59391 i |
| 50 | 2.40338 + 1.59391 i |
| 51 | 2.90065 - 1.45724 i |
| 52 | 2.90065 + 1.45724 i |

And the decimal approximation of $\tilde{\alpha}$ is

$$\text{N}\Big[\text{Root}\Big[131\,072 - 30\,081\,024\,\#1^{2} + 715\,784\,192\,\#1^{4} - 10\,181\,738\,496\,\#1^{6} + 83\,609\,604\,096\,\#1^{8} - 443\,259\,328\,512\,\#1^{10} + 1\,410\,471\,953\,408\,\#1^{12} - 1\,858\,643\,071\,488\,\#1^{14} + 18\,137\,673\,285\,920\,\#1^{16} - 14\,367\,112\,128\,688\,\#1^{18} + 56\,162\,265\,469\,488\,\#1^{20} - 73\,041\,229\,883\,512\,\#1^{22} + 73\,382\,345\,772\,378\,\#1^{24} - 122\,601\,623\,733\,111\,\#1^{26} + 73\,382\,345\,772\,378\,\#1^{28} - 73\,041\,229\,883\,512\,\#1^{30} + 56\,162\,265\,469\,488\,\#1^{32} - 14\,367\,112\,128\,688\,\#1^{34} + 18\,137\,673\,285\,920\,\#1^{36} - 1\,858\,643\,071\,488\,\#1^{38} + 1\,410\,471\,953\,408\,\#1^{40} - 443\,259\,328\,512\,\#1^{42} + 83\,609\,604\,096\,\#1^{44} - 10\,181\,738\,496\,\#1^{46} + 715\,784\,192\,\#1^{48} - 30\,081\,024\,\#1^{50} + 131\,072\,\#1^{52}\ \&,\ 7\Big]\Big]$$

0.0699128
